# Supplementary material for: Chiral structures and defects of lyotropic chromonic liquid crystals induced by saddle-splay elasticity
Source: arXiv:1504.03619 ancillary file (2015-05-07)
Supplement: Supplementary file 1 [file Supplementary_Info_Planar_Davidson_et_al.pdf]

# Supplemental information for "Chiral structures and defects of lyotropic chromonic liquid crystals induced by saddle-splay elasticity"

Zoey S. Davidson,[1] Louis Kang,[1] Joonwoo Jeong,[2] Tim Still,[1]
Peter J. Collings,[3,1] Tom C. Lubensky,[1] and A. G. Yodh[1]

[1]*Department of Physics & Astronomy,*
*University of Pennsylvania, Philadelphia, PA 19104, USA*
[2]*School of Natural Science, Department of Physics,*
*Ulsan National Institute of Science and Techonlogy (UNIST), Ulsan 689-798, Republic of Korea*
[3]*Department of Physics & Astronomy,*
*Swarthmore College, Swarthmore, PA 19081, USA*

(Dated: May 4, 2015)

**CONTENTS**


I. Theoretical notes on the escaped-twist (ET) configuration 2
A. Thermodynamic stability 2
1. Parallel axial configuration 2
2. ET configuration 3
B. Numerical configuration calculation of defects 3
C. Topological charge 4
D. Free energy approximation of defects for small $K_2$ 4
1. Domain wall 4
2. Point defect 5

II. Excluding azimuthal surface anchoring effects 6

III. Method of extracting angles from fluctuation movie 8

IV. Calculation of $K_{24}$ and its Error Bar 9

V. Jones Matrix Calculations 10
A. Defects 10
B. Comparison to Linear Twist 10

VI. Supplementary movie captions 13
A. Supplementary Movie 1: Raw director flickering 13
B. Supplementary Movie 2: Director flickering with time-average subtracted 13
C. Supplementary Movie 3: Fourier transform of the flickering amplitude 13
D. Supplementary Movie 4: Defect annihilation 13
E. Supplementary Movie 5: Point defect director rotation 13
F. Supplementary Movie 6: Nematic-Isotropic-Nematic transitions in a capillary 14

References 15


# I. THEORETICAL NOTES ON THE ESCAPED-TWIST (ET) CONFIGURATION

## A. Thermodynamic stability

To assess the stability of configurations, we set $\alpha(r) = \alpha_0(r) + \delta\alpha(r)$ and $\beta(r) = \beta_0(r) + \delta\beta(r)$, and expand the Frank free energy to quadratic order in small deviations $\delta\alpha$ and $\delta\beta$. Stability requires that the matrix of this quadratic form have only positive eigenvalues.

### *1. Parallel axial configuration*

The uniform parallel axial configuration has $\beta_0(r) = 0$. In this case, the nematic director and thus the entire free energy are independent of $\alpha$ to quadratic order. The Frank free energy becomes

$$\frac{F}{\pi L} = \frac{F_0}{\pi L} + \frac{1}{2\pi L}\int_0^R \mathrm{d}r\, \delta\beta M_{\beta\beta}\delta\beta. \tag{s.1}$$

We can solve the eigenvalue equation

$$M_{\beta\beta}\delta\beta = \lambda_\beta \delta\beta \tag{s.2}$$

subject to the boundary conditions of our system. We find that the $\lambda_\beta$'s are all positive for $K_{24} < 2K_2$ and that there exists a negative $\lambda_\beta$ for $K_{24} > 2K_2$. Thus, the parallel axial configuration is stable when it is the ground state and unstable when the ET configuration is the ground state. Note that the Ericksen stability condition $K_{24} < 2K_2$ is not violated by this uniform configuration.

*2. ET configuration*

We set $\alpha_0(r)$ and $\beta_0(r)$ to the ET configuration given by Eqs. (3) and (4) of the main text. This configuration only exists for $K_{24} > 2K_2$. The Frank free energy becomes

$$\frac{F}{\pi L} = \frac{F_0}{\pi L} + \frac{1}{2\pi L}\int_0^R \mathrm{d}r \begin{pmatrix} \delta\alpha & \delta\beta \end{pmatrix} \begin{pmatrix} M_{\alpha\alpha} & 0 \\ 0 & M_{\beta\beta} \end{pmatrix} \begin{pmatrix} \delta\alpha \\ \delta\beta \end{pmatrix}. \tag{s.3}$$

The stability matrix $\boldsymbol{M}$ is diagonal, so $\delta\alpha$ and $\delta\beta$ are decoupled. We can analytically and numerically solve the two eigenvalue equations

$$M_{\alpha\alpha}\delta\alpha = \lambda_\alpha\delta\alpha \quad \text{and} \quad M_{\beta\beta}\delta\beta = \lambda_\beta\delta\beta \tag{s.4}$$

subject to the boundary conditions of our system. We find that with $K_{24} > 2K_2$, the $\lambda_\alpha$'s and $\lambda_\beta$'s are all positive, so the ET configuration is stable. This violates the Ericksen stability condition $K_{24} < 2K_2$.

### B. Numerical configuration calculation of defects

To find the defect configurations, we use a relaxational method to minimize the Frank free energy $F$ (Eq. (1) in the main text). We introduce a time coordinate $t$ on which the director angles $\alpha(r,z,t)$ and $\beta(r,z,t)$ now depend (Eq. (2) and Fig. 1a in the main text). We provide initial guess $\alpha(r,z,0)$ and $\beta(r,z,0)$ and use the numerical method of lines to solve

$$\partial_t\alpha = -\Gamma_\alpha\frac{\delta F}{\delta\alpha} \quad \text{and} \quad \partial_t\beta = -\Gamma_\beta\frac{\delta F}{\delta\beta} \tag{s.5}$$

up to some $t_{\max}$ when $\alpha$, $\beta$ converge to solutions of the Euler-Lagrange equations. The $\Gamma$ factors are relaxational rates.

The domain of these defects span $0 \le r \le R$ and $-Z \le z \le Z$, where $R$ is the capillary radius and $Z$ is a large enough length so that the defect relaxes back to the bulk ET configuration. For $\alpha$, the boundary conditions for both smooth domain walls and point defects are the same: $\partial_r\alpha(0,z,t) = 0$ to satisfy stationarity of $F$, $\alpha(R,z,t) = \pi/2$ for homeotropic anchoring, and $\alpha(R,\pm Z,t) = \pi/2$ to match the bulk configuration. For $\beta$, stationary of $F$ enforces the natural boundary condition $R\partial_r\beta(R,z,t) = (K_{24}/2K_2 - 1/2)\sin 2\beta(R,z,t)$. For smooth domain walls, $\beta(0,z,t) = 0$; $\beta(r,\pm Z,t) = \pm\beta_{\mathrm{ET}}(r)$ gives a left-handed ($z<0$) to right-handed ($z>0$) defect and $\beta(r,\pm Z,t) = \mp\beta_{\mathrm{ET}}(r)$ gives a right-handed ($z<0$) to left-handed ($z>0$) defect. For point defects, $\beta(0,z,t) = \pi\Theta(-z)$, $\beta(r,-Z,t) = \pi - \beta_{\mathrm{ET}}(r)$, and $\beta(r,Z,t) = \beta_{\mathrm{ET}}(r)$ gives a left-handed ($z<0$) to right-handed ($z>0$) defect; $\beta(0,z,t) = \pi\Theta(z)$, $\beta(r,-Z,t) = \beta_{\mathrm{ET}}(r)$, and $\beta(r,Z,t) = \pi - \beta_{\mathrm{ET}}(r)$ gives a right-handed ($z<0$) to left-handed ($z>0$) defect. Here, $\beta_{\mathrm{ET}}$ is the ET configuration (Eq. (4) in the main text) and $\Theta$ is the Heaviside step function.

For better numerical convergence, a small cutoff ($10^{-15}R$) is used instead of 0 for the lower bound of $r$ near the central axis of the capillary. Also, for the point defect, we take $\beta(r,z,t) = \arctan[\frac{r}{z^3}b(r,z,t)]$ and minimize $F$ with respect to $b$ instead of $\beta$.

### C. Topological charge

The total topological charge inside a liquid crystal domain is [1]

$$d = \frac{1}{4\pi}\int_S \mathrm{d}u\,\mathrm{d}v\,\mathbf{n}\cdot(\partial_u\mathbf{n}\times\partial_v\mathbf{n}), \tag{s.6}$$

where $S$ is the 2D surface bounding the domain and parametrized by the coordinates $u$ and $v$. Taking the surface to be the boundary of a capillary domain $0 \le r \le R$, $-Z \le z \le Z$, and $0 \le \phi < 2\pi$, we calculate

$$d = \frac{\cos\beta(0,Z) - \cos\beta(0,-Z)}{2} \tag{s.7}$$

for any $\phi$-independent configuration that satisfies degenerate planar anchoring. Thus, domain walls have charge 0, left-handed ($z < 0$) to right-handed ($z > 0$) point defects have charge 1, and right-handed ($z < 0$) to left-handed ($z > 0$) point defects have charge $-1$. Liquid crystal topological charges are only consistent up to an overall sign; note that Eq. (s.6) is odd in $\mathbf{n}$ whereas director configurations are invariant under $\mathbf{n} \to -\mathbf{n}$.

### D. Free energy approximation of defects for small $K_2$

Here we make very rough analytical approximations of defect configurations and energies. We set $K_1 = K_3 \equiv K$, define $k_2 \equiv K_2/K$ and $k_{24} \equiv K_{24}/K$, and assume that $k_2 \ll 1$ and $k_2 \ll k_{24}$. We use dimensionless coordinates $s \equiv r/R$ and $w \equiv z/R$, and let $Z \to \infty$.

We first assume that $\alpha(s,w) = \pi/2$, a constant. The Frank free energy then only depends on $\beta$:

$$\frac{F}{\pi R K} = \int_0^1 \mathrm{d}s \int_{-\infty}^{\infty} \mathrm{d}w \left[k_2 s(\partial_s\beta)^2 + s(\partial_w\beta)^2 + k_2\frac{\sin^2 2\beta}{4s} + \frac{\sin^4\beta}{s}\right] - \int_{-\infty}^{\infty} \mathrm{d}w\,(k_{24}-k_2)\sin^2\beta(1,w). \tag{s.8}$$

#### 1. *Domain wall*

For a domain wall, we assume $\beta$ is separable inside the arctangent:

$$\beta(s,w) = \arctan\left[g(w)\frac{2\sqrt{k_2 k_{24}(k_{24}-2k_2)}\,s}{k_{24}-(k_{24}-2k_2)s^2}\right]. \tag{s.9}$$

This way, the natural boundary condition at $s = 1$ is always satisfied. We substitute this expression for $\beta$ into the Frank free energy Eq. (s.8) and expand in powers of $k_2$. To leading order, the defect free energy relative to the ET energy becomes

$$\frac{\Delta F}{\pi R K} = \frac{\pi}{4}\sqrt{k_2}\int_{-\infty}^{\infty}\mathrm{d}w\,\frac{(1-g)^2 + (\partial_w g)^2}{g}. \tag{s.10}$$

We need to solve the Euler-Lagrange equation

$$0 = (1-g)^2 - (\partial_w g)^2 \tag{s.11}$$

with the boundary condition $g(0) = 0$. This gives

$$g(w) = \mathrm{sgn}(w)\left(1 - \mathrm{e}^{-|w|}\right), \tag{s.12}$$

where $\mathrm{sgn}(w) = w/|w|$.

To get the energy, we have to substitute this $g(w)$ back into Eq. (s.8) to avoid a singularity at $w = 0$. Eventually, we get

$$\frac{\Delta F}{\pi R K} \approx \pi\sqrt{k_2}\log\frac{k_{24}}{\sqrt{k_2}}. \tag{s.13}$$

*2. Point defect*

We also assume that $\beta$ is separable, but the Euler-Lagrange equation Eq. (s.11) cannot be solved with the requisite boundary condition $g(w) \to \infty$ when $w \to 0^+$. So we adopt another strategy and take a similar separable $\beta$:

$$\beta(s, w) = \arctan\left[\frac{1}{g(w)}\frac{2\sqrt{k_2 k_{24}(k_{24} - 2k_2)}s}{k_{24} - (k_{24} - 2k_2)s^2}\right]. \tag{s.14}$$

We substitute this expression into the Frank free energy Eq. (s.8). The resulting integrand has a log-divergence at $g(w) \approx 0$ and is otherwise smooth. But it is comprised of diverging terms that precisely cancel and is thus not amenable to direct expansion. We adopt a different approach: we match the free energy density's behavior asymptotically around $g \approx 0$ and $g \approx 1$. In the latter case, we have to match leading powers of both small quantities $1 - g$ and $\partial_w g$. One empirical version that works is

$$\begin{aligned}\frac{\Delta F}{\pi R K} = \int_{-\infty}^{\infty} \mathrm{d}w \Bigg\{ &-\log\left[g(2-g)\right] - \left(\frac{1}{4k_2} + \frac{1}{2k_{24}}\right)\log\left[g(2-g)\right](\partial_w g)^2 - \left(1 - \frac{\pi}{4}\sqrt{k_2}\right)(1-g)^2 \\ &- \left(\frac{5 - 2\log 16k_2}{16k_2} + \frac{5 - 2\log 16k_2}{8k_{24}} + \frac{\pi}{4}\sqrt{k_2} + k_2\log 4k_2\right)(1-g)^2(\partial_w g)^2 \\ &+ \left(\frac{\pi}{4}\sqrt{k_2} + k_2\log 4k_2\right)(\partial_w g)^2 + \left(\frac{1 + \log 16k_2}{2} - \frac{\pi}{4}\sqrt{k_2}\right)(1-g)^4\Bigg\}\end{aligned} \tag{s.15}$$

Inspired by the domain wall case, we make the ansatz

$$g(w) = \mathrm{sgn}(w)\left(1 - \mathrm{e}^{-|w|/\xi}\right), \tag{s.16}$$

where $\xi$ is a characteristic defect length. Substituting this back into Eq. (s.15) and minimizing over $\xi$, we get

$$\xi = \sqrt{\frac{3 + 2\log 16k_2}{2\pi^2 - 9 + 3\log 16k_2}\frac{3}{8k_2}}. \tag{s.17}$$

For $k_2 = 0.1$, $\xi \approx 1.1$.

The minimum energy is, to leading orders in $k_2$,

$$\frac{\Delta F}{\pi R K} = \sqrt{\frac{(3 + 2\log 16k_2)(2\pi^2 - 9 + 3\log 16k_2)}{1536}}\left(\frac{3\pi}{2\pi^2 - 9 + 3\log 16k_2} + \frac{4}{\sqrt{k_2}} + \frac{4\sqrt{k_2}}{k_{24}}\right). \tag{s.18}$$

Note that for $k_2 \ll 1$ and $k_{24} \gtrsim 1$, the energy only weakly depends on $k_{24}$.

## II. EXCLUDING AZIMUTHAL SURFACE ANCHORING EFFECTS

The Frank saddle-splay free energy becomes in our case

$$\frac{F_{24}}{\pi L} = -K_{24} \sin^2 \beta_1, \tag{s.19}$$

where $K_{24}$ is the saddle-splay modulus, $\beta_1 = \beta(r = R)$ is the surface director angle, and $L$ is the length of the capillary. This energy takes a similar form to an anisotropic interfacial energy that favors planar alignment in the $\hat{\boldsymbol{\phi}}$-direction over the $\hat{\mathbf{z}}$-direction:

$$\frac{F_{\phi}}{\pi L} = -RW_{\phi} \sin^2 \beta_1, \tag{s.20}$$

where $W_{\phi}$ is the azimuthal alignment energy density and $R$ is the capillary radius.

We must exclude the possibility that some kind of azimuthal interfacial alignment energy is mimicking saddle-splay energy and affecting our measurement of $K_{24}$. Our experimental fit $K_{24}/K \approx 6.1$ and the measurement $K \approx 7\,\mathrm{pN}$ by [2] give $K_{24} \approx 50\,\mathrm{pN}$. Thus, for an azimuthal alignment effect to interfere with our measurement, it must have $RW_{\phi} \gtrsim 50\,\mathrm{pN}$. We expect a very small $W_{\phi}$ because as discussed in the main text, examination of the capillary surface under atomic force microscopy (AFM) and scanning electron microscopy (SEM) reveals no microscopic structures that could favor anisotropic alignment (see Fig. s1). Anisotropic surface alignment is commonly achieved by rubbing the surface with an abrasive pad, which produces large grooves along which the surface director prefers to be oriented. We measured the surface profile of rubbed glass prepared as in Ref. [3] and found large grooves in the glass surface (see Fig. s2). This technique gives $W_{\phi} \approx 3 \times 10^{-7}\,\mathrm{J\,m^{-2}}$ for Sunset Yellow (SSY) [3], which for a 100 µm-capillary, would correspond to $RW_{\phi} \approx 30\,\mathrm{pN}$. With no alignment structures visible, we expect our capillary to have $RW_{\phi} \ll 30\,\mathrm{pN}$. Thus, $RW_{\phi}$ is insigificant compared to $K_{24}$, and anisotropic surface alignment effects can be ignored.

We also carried out temperature-dependent experiments in which we evolved the sample in the capillary from nematic phase to isotropic phase and then back to the nematic phase. These studies (see section VI F and its movie) demonstrated that entirely new defects were produced in very different locations and that the same general configurations of left and right-handed ET are recovered. Importantly in this study, the same textures did not recover to the same place prior to the heating and cooling cycle. This finding indicates that anchoring anisotropy (even if it exists) is too weak to affect preference for one handedness of ET over the other. Since we also always find the director at the capillary surface to be close to but less than 90 degrees from the capillary axis, regions of handedness different from those prior to heating further indicates no easy access is imprinted on the capillary surface.

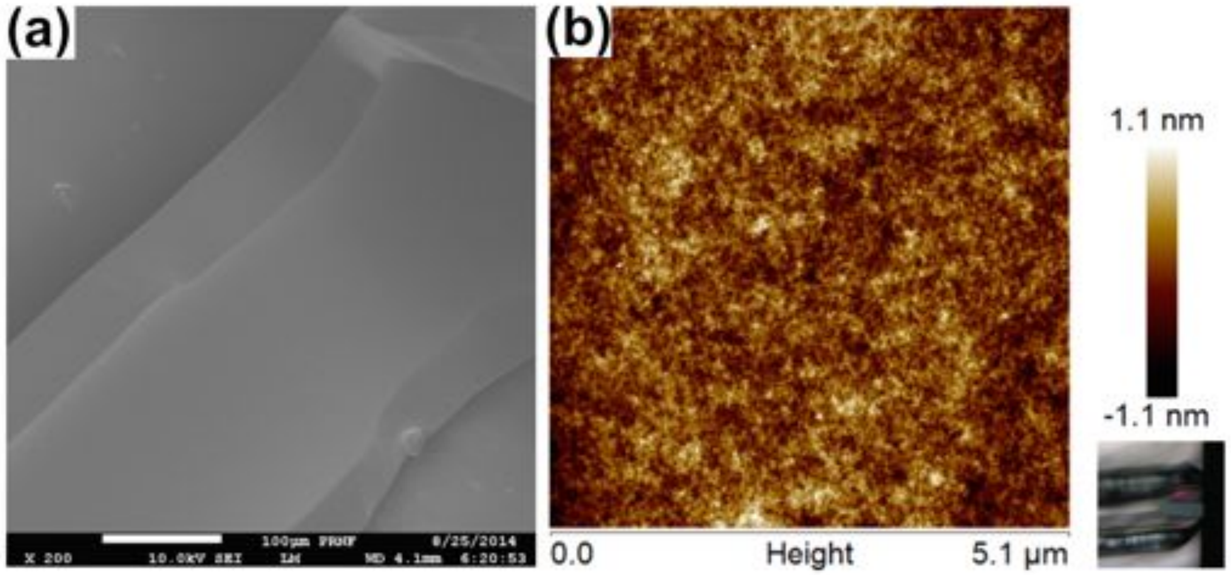


FIG. s1. **(a)** SEM of a broken glass capillary with silver sputter coating shows no aligning features. **(b)** AFM height map of a broken capillary shows a smooth surface to within ±1.1 nm with surface roughness 0.3 nm (RMS) after subtraction of overall curvature. Inset is a video still of AFM cantilever inside a capillary.

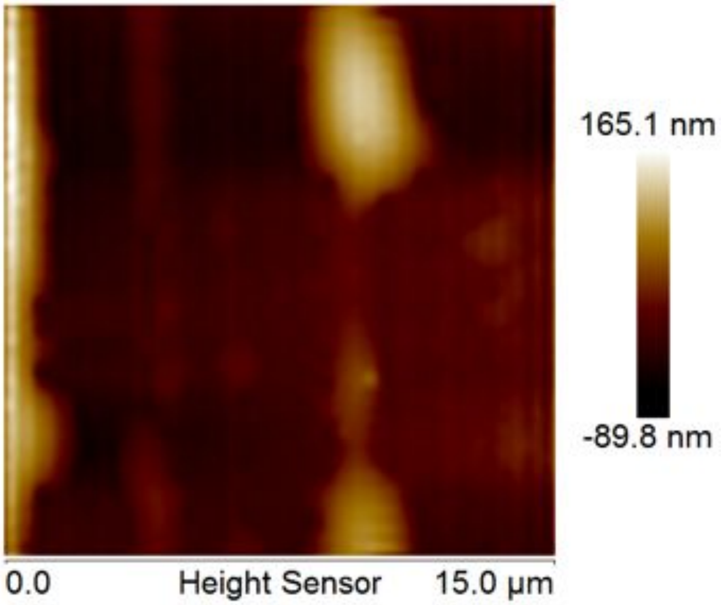


FIG. s2. AFM height map of a rubbed glass slide prepared as in Ref. [3]. The height map shows ridges running along the rubbed direction. The surface roughness is 27 nm (RMS).

There is a possibility that azimuthal surface alignment could be favored by a surface anchoring energy that couples the director to the curvature tensor, which has been proposed in models of deformable membranes [4, 5] but has never been directly experimentally observed in LC systems to our knowledge. Such a symmetry-allowed anchoring energy would look like

$$F_w = \frac{w}{2} \int \mathrm{d}^2 S \, n_i n_j L_{ij}, \tag{s.21}$$

where $i$ and $j$ are coordinate indices in 3D space, $\mathrm{d}^2S$ is the magnitude of the surface area element, and $L_{ij} = -\partial_i \nu_j$ is the surface curvature tensor, or second fundamental form, in the 3D basis. $\boldsymbol{\nu}$ is the outward-pointing normal to the surface. (Perhaps a more common form for $\boldsymbol{L}$, as described in Ref. [6], uses a local 2D basis of surface tangent vectors $\hat{\mathbf{e}}_1$ and $\hat{\mathbf{e}}_2$: $L_{\alpha\beta} = e_{\alpha i} e_{\beta j} L_{ij}$, where $\alpha$ and $\beta$ indicate the basis vector index 1 or 2.) Using our parametrization for $\mathbf{n}$ and taking our surface to be a cylinder of radius $R$ and length $L$, we get

$$\frac{F_w}{\pi L} = -w \sin^2 \beta_1, \tag{s.22}$$

which is identical to Eq. s.19 with $K_{24}$ replaced by the anchoring strength $w$. Note that unlike the traditional Rapini-Papoular energy (Eq. s.20), the cylinder radius $R$ scales out of this energy. In fact, we can show that for degenerate planar boundary conditions, $K_{24}$ precisely couples the nematic director to the curvature tensor just like this anchoring term. We rewrite the $K_{24}$ term of Eq. 1 in the main text in an equivalent manner and use both $\boldsymbol{\nu} \cdot \mathbf{n} = 0$ and $\partial_j(\nu_i n_i) = 0$, where again $\boldsymbol{\nu}$ is the surface normal, to obtain

$$\begin{aligned} F_{24} &= -\frac{K_{24}}{2} \int \mathrm{d}^3\mathbf{x}\, \boldsymbol{\nabla} \cdot (\mathbf{n} \times \boldsymbol{\nabla} \times \mathbf{n} + \mathbf{n} \boldsymbol{\nabla} \cdot \mathbf{n}) \\ &= \frac{K_{24}}{2} \int \mathrm{d}^3\mathbf{x}\, \boldsymbol{\nabla} \cdot [(\mathbf{n} \cdot \boldsymbol{\nabla})\mathbf{n} - \mathbf{n} \boldsymbol{\nabla} \cdot \mathbf{n}] \\ &= \frac{K_{24}}{2} \int \mathrm{d}^2S\, \boldsymbol{\nu} \cdot (\mathbf{n} \cdot \boldsymbol{\nabla})\mathbf{n} \\ &= \frac{K_{24}}{2} \int \mathrm{d}^2S\, \nu_i n_j \partial_j n_i \\ &= -\frac{K_{24}}{2} \int \mathrm{d}^2S\, n_i n_j \partial_j \nu_i \\ &= \frac{K_{24}}{2} \int \mathrm{d}^2S\, n_i n_j L_{ij}. \end{aligned} \tag{s.23}$$

Thus, saddle-splay energy and curvature-coupled surface anchoring energy have the same mathematical form for systems with degenerate planar boundary conditions. The only difference between the two effects is their microscopic origin. Saddle-splay energy arises solely from energetic and entropic interactions among LC molecules/mesogens themselves due to confinement into a curved geometry; it is independent of the identity of the confining container. An anchoring energy must arise from energetic interactions between LC molecules/mesogens and the confining container; presumably, changing the surface chemistry of the container can change the magnitude and/or sign of this energy.

## III. METHOD OF EXTRACTING ANGLES FROM FLUCTUATION MOVIE

To carry out the flickering measurements, the sealed sample capillary was placed on an indium tin oxide (ITO) coated slide. The ITO slide was attached to a proportional-integral-derivative temperature controller used to maintain sample temperature. The sample was then coated with index matching oil before being sandwiched between the slide and oil-objective. The sample was typically illuminated between crossed-polarizers by quasi-monochromatic light from a 660 nm LED light (ThorLabs LED4D067) that was passed through a 660 nm (FWHM = 10 nm) band pass filter in a Köhler configuration. The condenser diaphragm was narrowed to maximize contrast and parallel illumination.

Images were captured in black and white by a Uniq UP680-CL video camera; the camera gain and shutter speed were adjusted to maximize dynamic range and fluctuation contrast. We use

160x total magnification for narrow depth of focus and high spatial resolving power of director field fluctuations. A piezo-objective-positioner enabled us to precisely move the image plane radially through the capillary; at each position (i.e., for each image plane position) we record movies of the director field fluctuations. The image planes are obtained at one micron intervals. Movies were cropped to a narrow region of 10% of the capillary diameter (see Supplementary Information mov. 1). At each image plane, we determined the time-average of the video image sequence; then we subtracted the time-average from every frame in order to resolve only the fluctuations. An example of a single frame (with subtraction) is in main text figure 3a (for the full video, see Supplementary Information mov. 2).

A Hann-windowed fast Fourier transform was computed for the subtracted image associated with every frame. The time-average of these subtracted images was then used to derive the dominant direction of scattering; the latter was accomplished by fitting a two-dimensional Gaussian to the averaged Hann-windowed fast Fourier transform (see figure 3b in main text). The dominant direction so-determined is perpendicular to the local nematic director in the sample plane [7]. Repeated measurements at different depths in the capillary gives us $\beta(r)$ (see Supplementary Information mov. 3).

## IV. CALCULATION OF $K_{24}$ AND ITS ERROR BAR

The flickering experiment was performed five times (see table s.I) in five different capillaries with diameters ranging from 88 µm to 99 µm. The value of $K_{24}/K_3$ is a fitting parameter in the nonlinear least squares fit (NLLS) to $\beta(r/R)$ (see Eq. (4) of main text). In each experiment a sequence of $\beta_i$ are determined at image slice position, $r_i$, in the capillary. Note also, the $r_i$ of each experiment are scaled to the measured value of the capillary radius, $R$, of the particular experiment. The capillary radii were measured using a 100x magnification with a wider field-of-view so that the whole capillary was captured in each image. The diameter at mid-plane was determined from the image by comparison to a standardized micrometer scale. Uncertainties arose due to the finite pixel size and our limited ability to choose the image plane that corresponded to the capillary diameter (as opposed to a capillary chord). Together these sources of error led to an experimental uncertainty in the capillary radius of $\pm 400$ nm.

Error propagation due to uncertainties in capillary radius are somewhat unusual for these experiments. For example, if $R$ of a particular flickering data set is replaced by a slightly larger radius (e.g., $R + 400$ nm), then the extrapolated angle $\beta_1$ will increase, and since $K_{24}$ is proportional to $\tan(\beta_1)$, a measurement error due to a slightly larger capillary $R$ results in a substantial (positive) shift in the best-fit value of $K_{24}/K_3$ when $\beta_1$ is nearing $\pi/2$. On the other hand, if $R$ is replaced by a slightly smaller radius (e.g., $R - 400$ nm), then the measurement error produces a comparatively smaller (negative) shift in the best-fit value of $K_{24}/K_3$. The measurement error bars are thus asymmetric about the mean.

The $K_{24}/K_3$ data for each capillary are presented in Table s.I. The three columns correspond to $K_{24}/K_3$ obtained using our best estimate of $R$ for each experiment (first column), and $K_{24}/K_3$ obtained using the smallest (second column) and largest (third column) $R$ due to the limited measurement resolution.

The average and standard deviation of our date derived using the best estimate of $R$ is $\overline{K_{24}/K_3} = 6.6$; the standard deviation is $\sigma_{K_{24}/K_3} = 2.8$ giving a bounding interval $[3.8, 9.4]$. These are the numbers we report in the main text.

Of course, the distributions may not be symmetric, and there are many other ways to estimate $K_{24}/K_3$. Therefore, as a check, we computed $\overline{K_{24}/K_3}$, etc., using several different statistical models. A second model used a weight for each experiment set by $K_{24}/K_3$ divided by the difference

| $K_{24}/K_3$ | Lower Bound $K_{24}/K_3$ | Upper Bound $K_{24}/K_3$ |
|---|---|---|
| 6.48 | 4.74 | 10.32 |
| 8.07 | 3.6 | 28.59 |
| 10.5 | 4.37 | 24.3 |
| 3.75 | 2.54 | 7.21 |
| 4.03 | 3.13 | 5.681 |

TABLE s.I. NLLS fit parameters and uncertainty from five independent flickering measurements. Upper and lower bounds reflect refitting after replacing $R$ by by $R + 400$ nm and $R - 400$ nm, respectively.

between the upper and lower bounds for $K_{24}/K_3$; a third model used a weight for each experiment equal to the difference between the upper and lower bounds for $K_{24}/K_3$; a fourth model computed the means of each the three columns in the table above to define the error interval; a fifth model employed the log-transform of the data in the table. All of these models gave means and error-intervals that were overlapping with the simplest approach. If we average the results from all of these methods to generate a method-averaged mean and error interval, then we obtained $\overline{K_{24}/K_3} = 5.8$ and a bounding interval of $[3.5, 10.0]$.

The parameter $K_2/K_3$ is a much stiffer parameter with respect to both the NLLS fit and the capillary size, so across measurements we simply calculate an average value $\overline{K_2/K_3} = 0.12$ with $\sigma_{K_2/K_3} = 0.04$. Thus we find $K_{24}/K_2 \approx 55.0$.

## V. JONES MATRIX CALCULATIONS

### A. Defects

Experimental polarized optical microscopy images of point defects in the samples under monochromatic illumination were compared to simulated 2D transmittance profiles as in main text Fig. 4a. Simulated images were computed using LC director field models calculated as in supplementary information I B, and with known optical components (polarizers and a full-wave plate), using $2 \times 2$ Jones matrices as in [8, 9]. See Fig. s3 and Fig. s4 for additional examples in capillaries of 50µm and 138µm respectively.

### B. Comparison to Linear Twist

Far from defects, we also compared polarized optical microscopy textures of the LCLC in capillary confinement to Jones matrix images of both an ET configuration model and linear twist configuration model as in Ref. [10]. We find for the total twist angle found by a director flickering experiment, the ET Jones matrix images reproduce the features better than a linear twist model as in Fig. s5. For example, the bright lines near the capillary edges when the capillary is along one of the polarizer directions or the thickness of the stripes when the capillary is at 45° to the polarizer directions are reproduced by the ET model and not the linear twist model.

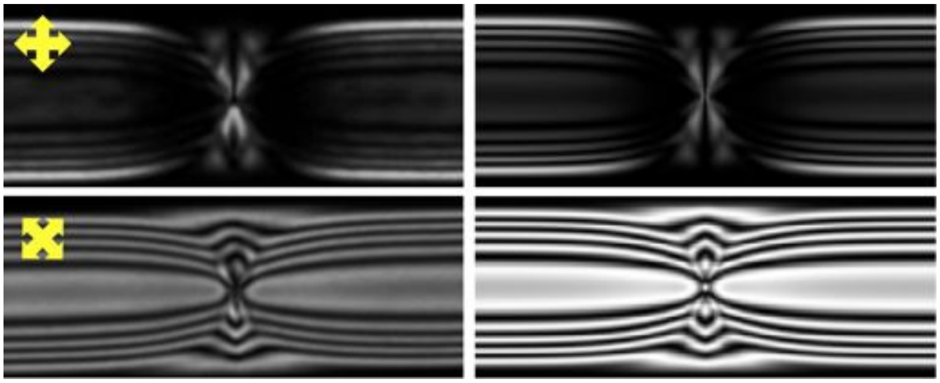

FIG. s3. Left side, monochromatic, 660 nm, cross polarized images of 30 % wt./wt. SSY at 25°C in a 50µm diameter capillary. Right side the corresponding Jones Matrix computed images with $\beta_1 = 85°$. Polarizer and analyzer orientation indicated by crossed yellow double arrows.

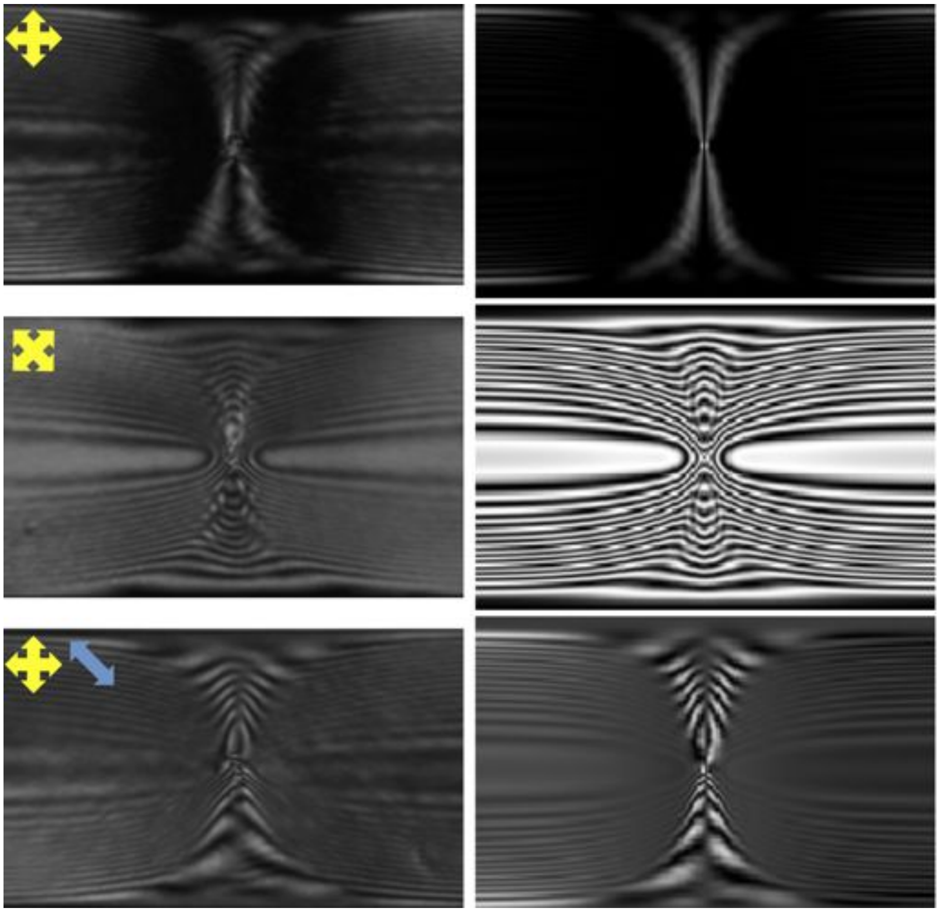

FIG. s4. Left side, monochromatic, 660 nm, cross polarized images of 30 % wt./wt. SSY at 25°C in a 138µm diameter capillary. Right side the corresponding Jones Matrix computed images with $\beta_1 = 85°$. Polarizer and analyzer orientation indicated by crossed yellow double arrows. Single blue double arrow indicates full-wave plate (optical path difference $\sim$ 550 nm). The full-wave plate distinguishes between regions of opposite handedness.

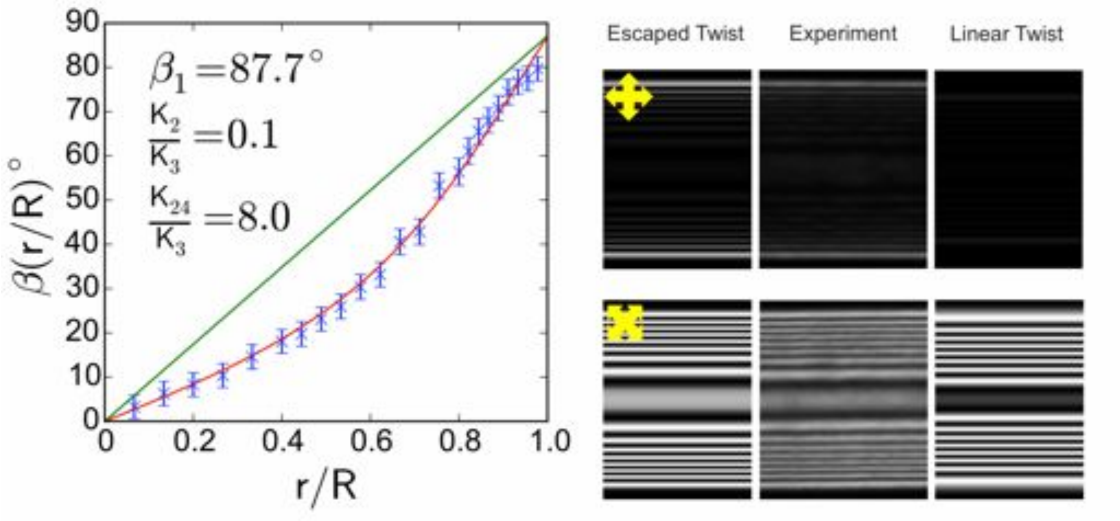


FIG. s5. Left side, the results of a director flickering experiment from a 92 µm diameter capillary. The green line indicates the profile of a linear twist with the same angle at the capillary surface as that of the fit, 87.7°. Right side, the corresponding Jones Matrix computed images with $\beta_1 = 87.7°$ from the ET model, the experiment, and the linear twist model. Monochromatic 660 nm light, and birefringence of -0.066. Polarizer and analyzer orientation indicated by crossed yellow double arrows.

## VI. SUPPLEMENTARY MOVIE CAPTIONS

### A. Supplementary Movie 1: Raw director flickering

Sample director flickering real-time movie between crossed polarizers at a constant focal plane cropped to a 38.4 µm x 38.4 µm area. See Sec. III for detailed experimental methods.

### B. Supplementary Movie 2: Director flickering with time-average subtracted

The time-average of Supplementary Movie 1 was subtracted from every frame of Supplementary Movie 1. This movie plays in real time and corresponds to a 38.4 µm x 38.4 µm area.

### C. Supplementary Movie 3: Fourier transform of the flickering amplitude

At each focal plane along the capillary radius, a flickering movie was taken and its time-average was subtracted from every frame. We performed a 2D Hann-windowed fast Fourier transform on each subtracted image and time-averaged the results. The movie starts at a focal plane close to the capillary center and ends beyond the inner capillary surface. Contours indicate constant values of the 2D Gaussian fit performed at each focal plane.

### D. Supplementary Movie 4: Defect annihilation

Supplementary Movie 4 is speeded up $\sim 2700\times$ and imaged with crossed polarizers and a full wave plate. The temperature was held at 33C to lower the viscosity and make this observation more likely. There are several effects that occur within this movie. Debris in the sample enters into view from the right side and is attracted to and attaches to the right most defect. Over the course of the movie, the central brightness varies greatly. It is likely the concentration increases due to slight evaporation of water from the capillary. Finally, at $\sim$ 28s, the two defects on the left annihilate. The annihilating defects leave behind debris they had trapped at their core.

### E. Supplementary Movie 5: Point defect director rotation

Chiral point defects as global rotations of classic achiral hedgehogs. We first plot the director configuration of two point defects corresponding to a classic radial hedgehog and a classic hyperbolic hedgehog separating achiral nematic domains. The azimuthal director angle is $\alpha(r, z) = 0$. We then perform a global rotation of the director field about the $z$-axis through $2\pi$ radians, i.e., we let $\alpha(r, z) = \alpha$ increase homogeneously from 0 to $2\pi$. At $\alpha = \pi/2$, the radial hedgehog becomes approximately the chiral right-to-left defect and the hyperbolic hedgehog becomes approximately the chiral left-to-right defect. They separate ET domains of alternating handedness. At $\alpha = \pi$, the original hedgehogs switch identities and the system loses all local chirality. At $\alpha = 3\pi/2$, the director configuration becomes a mirror image of the $\alpha = \pi/2$ configuration. Finally, at $\alpha = 2\pi$, the system returns to its original configuration. Topological charge is conserved throughout this transformation, so our movie demonstrates that chiral point defects have charge $\pm 1$, with opposite signs for defects of opposite chirality. The overall sign is not well-defined, as discussed in [1] and illustrated by this movie; it can be set by choosing one of the two physically equivalent directions for the director at one location.

### F. Supplementary Movie 6: Nematic-Isotropic-Nematic transitions in a capillary

A section of a 100 µm capillary filled with SSY initially in the nematic phase is heated to the fully isotropic phase, and then cooled back to the nematic phase. The locations of defects and regions of opposite ET handedness change position along the capillary axis indicating that there is no preference for one handedness over another or that there is a memory imparted on the capillary surface between cycles of heating and cooling. This movie is speed up $\sim 40\times$ and imaged with crossed polarizers and a full wave plate in quasi-monochromatic.

[1] G. P. Alexander, B. G. Chen, E. A. Matsumoto, and R. D. Kamien, Rev. Mod. Phys. **84**, 497 (2012).
[2] S. Zhou, Y. A. Nastishin, M. M. Omelchenko, L. Tortora, V. G. Nazarenko, O. P. Boiko, T. Ostapenko, T. Hu, C. C. Almasan, S. N. Sprunt, J. T. Gleeson, and O. D. Lavrentovich, Phys. Rev. Lett. **109**, 037801 (2012).
[3] C. K. McGinn, L. I. Laderman, N. Zimmermann, H.-S. Kitzerow, and P. J. Collings, Phys. Rev. E **88**, 062513 (2013).
[4] P. Biscari and E. M. Terentjev, Phys. Rev. E **73**, 051706 (2006).
[5] Y. K. Murugesan, D. Pasini, and A. D. Rey, Soft Matter **7**, 7078 (2011).
[6] R. D. Kamien, Rev. Mod. Phys. **74**, 953 (2002).
[7] P. G. de Gennes and J. Prost, *The Physics of Liquid Crystals* (Clarendon Press, 1995).
[8] J. Jeong, Z. S. Davidson, P. J. Collings, T. C. Lubensky, and A. G. Yodh, Proc. Nat. Acad. Sci. **111**, 1742 (2014).
[9] J. Jeong, L. Kang, Z. S. Davidson, P. J. Collings, T. C. Lubensky, and A. G. Yodh, Proc. Nat. Acad. Sci. , 201423220 (2015).
[10] V. Koning, B. C. van Zuiden, R. D. Kamien, and V. Vitelli, Soft Matter **10**, 4192 (2014).
